# Supplementary material for: Leveraging Schema Labels to Enhance Dataset Search
Source: arXiv:2001.10112 source file (2020-01-27)
Supplement: Supplementary file 1 [file appendix.tex]

%%%% FILE NOT USED NOW %%%%

\appendix
%\newpage
\section{Task Descriptions}\label{append}

% Please add the following required packages to your document preamble:
% \usepackage[normalem]{ulem}
% \useunder{\uline}{\ul}{}
% Please add the following required packages to your document preamble:
% \usepackage[normalem]{ulem}
% \useunder{\uline}{\ul}{}
\begin{table*}[h]
\begin{tabular}{|c|l|}
\hline
Task Number & \multicolumn{1}{c|}{Task Description} \\ \hline
1 & \begin{tabular}[c]{@{}l@{}}In order to design a wind energy conversion system in Kansas,  a company needs the monthly wind\\ speeds in Kansas between 2003-2004. As an employee of the company, you are asked to write a query\\ to find such datasets. Relevant results should include monthly wind speed in Kansas between\\ 2003-2004. Datasets that contain the wind speed of areas within Kansas are also relevant.\end{tabular} \\ \hline
2 & \begin{tabular}[c]{@{}l@{}}To review the effectiveness of the National School Lunch Program (NSLP), a team wants to find out\\ how many and which schools have participated in the program, and how many meals have been served\\ in each of these schools. As one of the team members, you are asked to write a query to find \\ datasets that could help the review process.\end{tabular} \\ \hline
3 & \begin{tabular}[c]{@{}l@{}}A researcher is planning to study the economic development of Peru. Specifically, the researcher\\ requires the population of in Peru from 1986-94 for analysis. Please write a query to help the\\ researcher find datasets containing such information.\end{tabular} \\ \hline
4 & \begin{tabular}[c]{@{}l@{}}A journalist needs background on how the finance industry has changed in Texas in recent years.\\ The reporter wants to find banks that have failed in Texas in the past ten years.  Write a query\\ to help the journalist find such datasets.\end{tabular} \\ \hline
5 & \begin{tabular}[c]{@{}l@{}}A veterans advocacy group wants to collect data on federal spending in order to determine which\\ issues they need to focus their efforts on. They have not yet found how much is spent on medical\\ care in the state of Mississippi by the Department of Veterans Affairs. Write a query to help them\\ datasets containing the information needed.\end{tabular} \\ \hline
6 & \begin{tabular}[c]{@{}l@{}}A public policy expert is interested in trends in electricity pricing. The expert needs to know how\\ the price of electricity has changed in the Western region of the U.S. over time. Write a query to\\ help the expert find datasets that will contain useful information.\end{tabular} \\ \hline
\end{tabular}
\caption{Task descriptions used in the creation of the Federal Datasets Corpus.}
\end{table*}
